# Supplementary material for: Why do tree-based models still outperform deep learning on tabular data?
Source: arXiv:2207.08815 source file (2022-07-18)
Supplement: Supplementary file 1 [file supplementary.tex]

\appendix

\section{Appendix}

Include extra information in the appendix. This section will often be part of the supplemental material. Please see the call on the NeurIPS website for links to additional guides on dataset publication.

\begin{enumerate}

\item Submission introducing new datasets must include the following in the supplementary materials:
\begin{enumerate}
  \item Dataset documentation and intended uses. Recommended documentation frameworks include datasheets for datasets, dataset nutrition labels, data statements for NLP, and accountability frameworks.
  \item URL to website/platform where the dataset/benchmark can be viewed and downloaded by the reviewers.
  \item Author statement that they bear all responsibility in case of violation of rights, etc., and confirmation of the data license.
  \item Hosting, licensing, and maintenance plan. The choice of hosting platform is yours, as long as you ensure access to the data (possibly through a curated interface) and will provide the necessary maintenance.
\end{enumerate}

\item To ensure accessibility, the supplementary materials for datasets must include the following:
\begin{enumerate}
  \item Links to access the dataset and its metadata. This can be hidden upon submission if the dataset is not yet publicly available but must be added in the camera-ready version. In select cases, e.g when the data can only be released at a later date, this can be added afterward. Simulation environments should link to (open source) code repositories.
  \item The dataset itself should ideally use an open and widely used data format. Provide a detailed explanation on how the dataset can be read. For simulation environments, use existing frameworks or explain how they can be used.
  \item Long-term preservation: It must be clear that the dataset will be available for a long time, either by uploading to a data repository or by explaining how the authors themselves will ensure this.
  \item Explicit license: Authors must choose a license, ideally a CC license for datasets, or an open source license for code (e.g. RL environments).
  \item Add structured metadata to a dataset's meta-data page using Web standards (like schema.org and DCAT): This allows it to be discovered and organized by anyone. If you use an existing data repository, this is often done automatically.
  \item Highly recommended: a persistent dereferenceable identifier (e.g. a DOI minted by a data repository or a prefix on identifiers.org) for datasets, or a code repository (e.g. GitHub, GitLab,...) for code. If this is not possible or useful, please explain why.
\end{enumerate}

\item For benchmarks, the supplementary materials must ensure that all results are easily reproducible. Where possible, use a reproducibility framework such as the ML reproducibility checklist, or otherwise guarantee that all results can be easily reproduced, i.e. all necessary datasets, code, and evaluation procedures must be accessible and documented.

\item For papers introducing best practices in creating or curating datasets and benchmarks, the above supplementary materials are not required.
\end{enumerate}

\subsection{Remark on the hyper parameter tuning }
 We claimed that tree-based models' are superior for every random search budget, and the performance gap stays wide even after a large number of random search iteration. However, this might not longer be true when adding additional regularization technique to our random search, such as data augmentation. Indeed, \cite{kadraWelltunedSimpleNets2021} find that searching through a "cocktail" of regularization on a Multi-Layer-Perceptron is competitive with XGBoost after half an hour of tuning (for both models), though the datasets considered in their paper are quite different, in particular with the presence of "deterministic" game-inspired datasets in \cite{kadraRegularizationAllYou2021}, on which their method performs very well.
\subsection{Datasets used}\label{supp:datasets}
Make tables

\subsection{More benchmarks}\label{supp:benchmarks}

\paragraph{Large-sized datasets}

\begin{figure}
\centering
\begin{subfigure}{.5\textwidth}
  \centering
  \includegraphics[width=\linewidth]{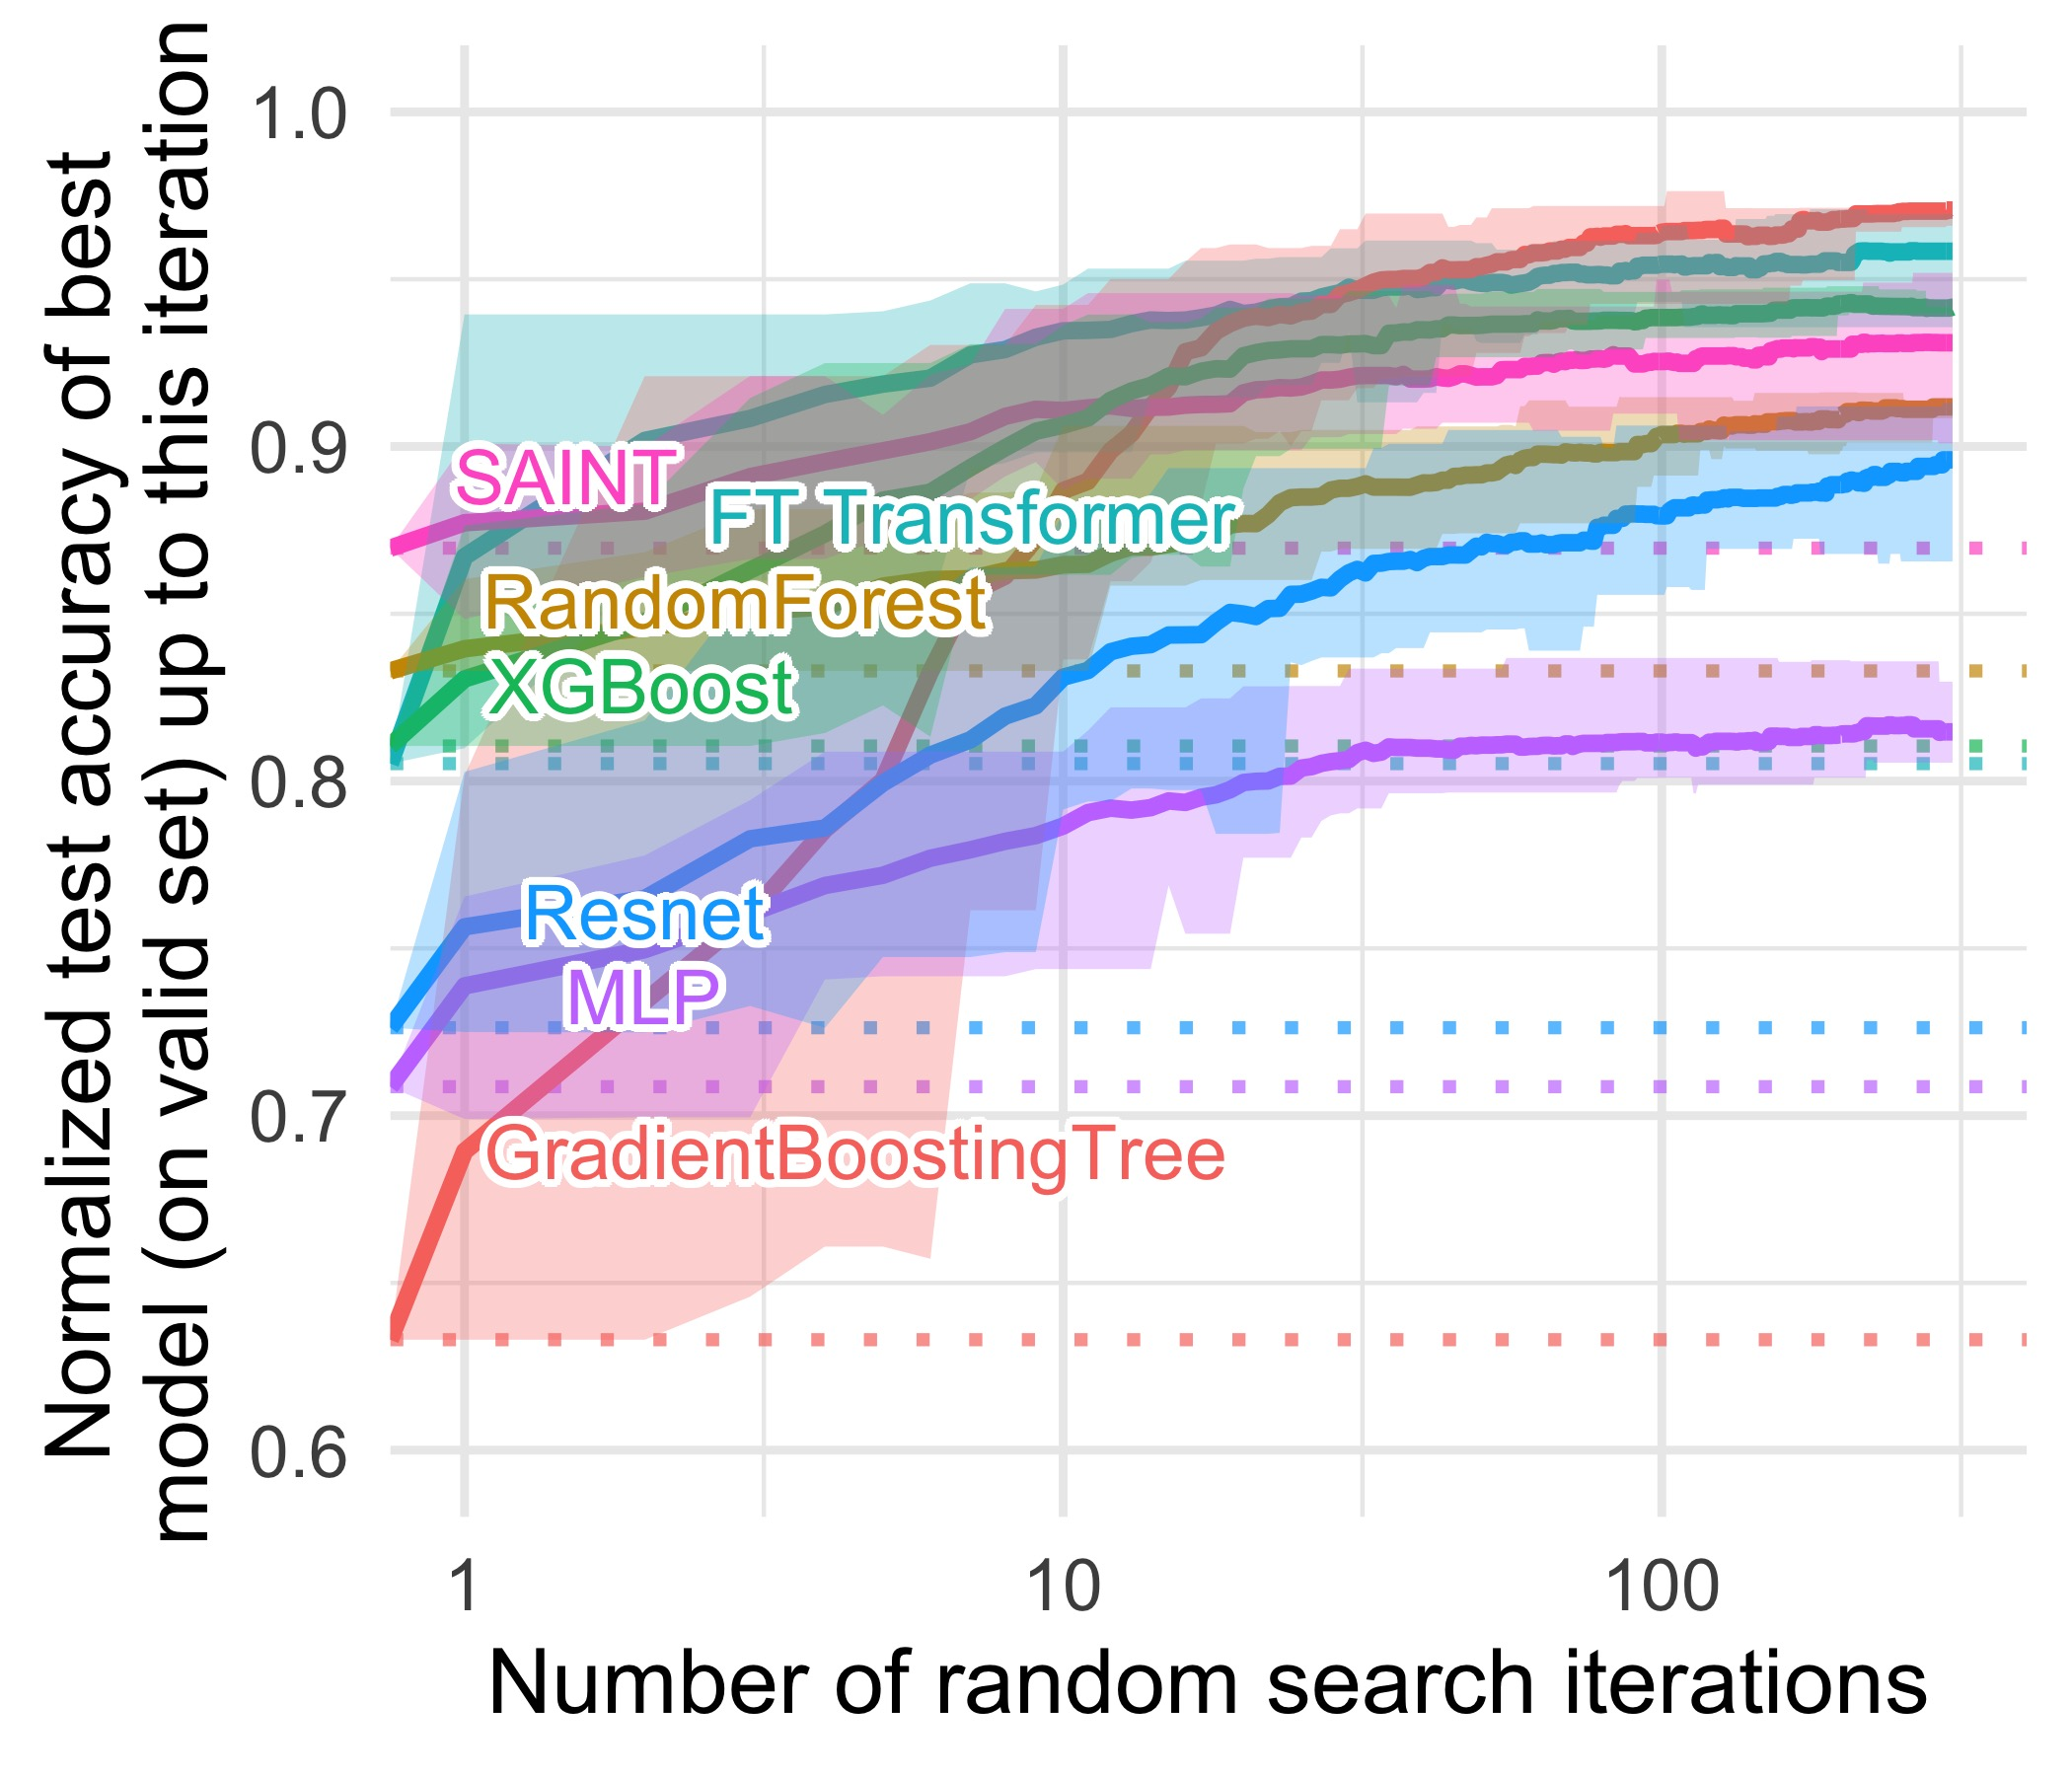}   
  \caption{Classification. WARNING: only on 4 datasets, 3 of which already in the FT Transformer paper.}
  \label{fig:benchmark_categorical_classif_large}
\end{subfigure}%
\begin{subfigure}{.5\textwidth}
  \centering
  \caption{Regression}
  \label{fig:benchmark_categorical_regression_large}
\end{subfigure}
\caption{\textbf{Benchmark on large-sized datasets, with only numerical features}. Dotted lines correspond to the score of the default hyperparameters, which is also the first random search iteration. Each value corresponds to the test score of the best model (on the validation set) after a specific number of random search iterations, averaged on 15 shuffles of the random search order. The ribbon corresponds to the minimum and maximum scores on these 15 shuffles.}
\label{fig:benchmark_categorical_large}
\end{figure}

\begin{figure}
\centering
\begin{subfigure}{.5\textwidth}
  \centering
  \caption{Classification}
  \label{fig:benchmark_categorical_classif_large_2}
\end{subfigure}%
\begin{subfigure}{.5\textwidth}
  \centering
  \caption{Regression}
  \label{fig:benchmark_categorical_regression_large_2}
\end{subfigure}
\caption{\textbf{Benchmark on medium-sized datasets, with both numerical and categorical features}. Dotted lines correspond to the score of the default hyperparameters, which is also the first random search iteration. Each value corresponds to the test score of the best model (on the validation set) after a specific number of random search iterations, averaged on 15 shuffles of the random search order. The ribbon corresponds to the minimum and maximum scores on these 15 shuffles.}
\label{fig:benchmark_categorical_large_2}
\end{figure}

\subsection{More details on benchmark}\label{supp:benchmark_details}

\paragraph{Number of folds}

For each dataset and hyperparameters combination, we vary the number of folds used for our algorithms evaluation depending on the number of testing samples:

\begin{itemize}
 \item If We have more than 6000 samples, we evaluate our algorithms on 1 fold.
 \item If we have between 3000 and 6000 samples, we evaluate our algorithms on 2 folds.
 \item If we have between 1000 and 3000 samples, we evaluate our algorithms on 3 folds.
 \item If we have less than 1000 testing samples, we evaluate our algorithms on 5 folds.
\end{itemize}

Every algorithms and hyperparameters combinations are evaluated on the same folds.

\paragraph{Hardware}
GPU models
measure time difference?

\subsection{More details on experiments}\label{supp:xp_details}
In this section, we give more details on the choices we had to make when creating our experiments. As aggregated results can sometimes be hard to interpret, we also show the results of each experiment on each dataset.

\paragraph{High-frequency}

Details:

\begin{itemize}
    \item We restrict all datasets to their 5 most important features (according to a RandomForest feature importance ranking). This makes the smoothing easier, as kernel smoothing can be hard in high-dimension, while keeping enough features to produce interesting results.
    \item We estimate the covariance matrix of these features though ScikitLearn's MinCovDet, which is more robust to outliers than the emprical covariance.
\end{itemize}

\begin{figure}
    \centering
    \includegraphics[scale=0.1]{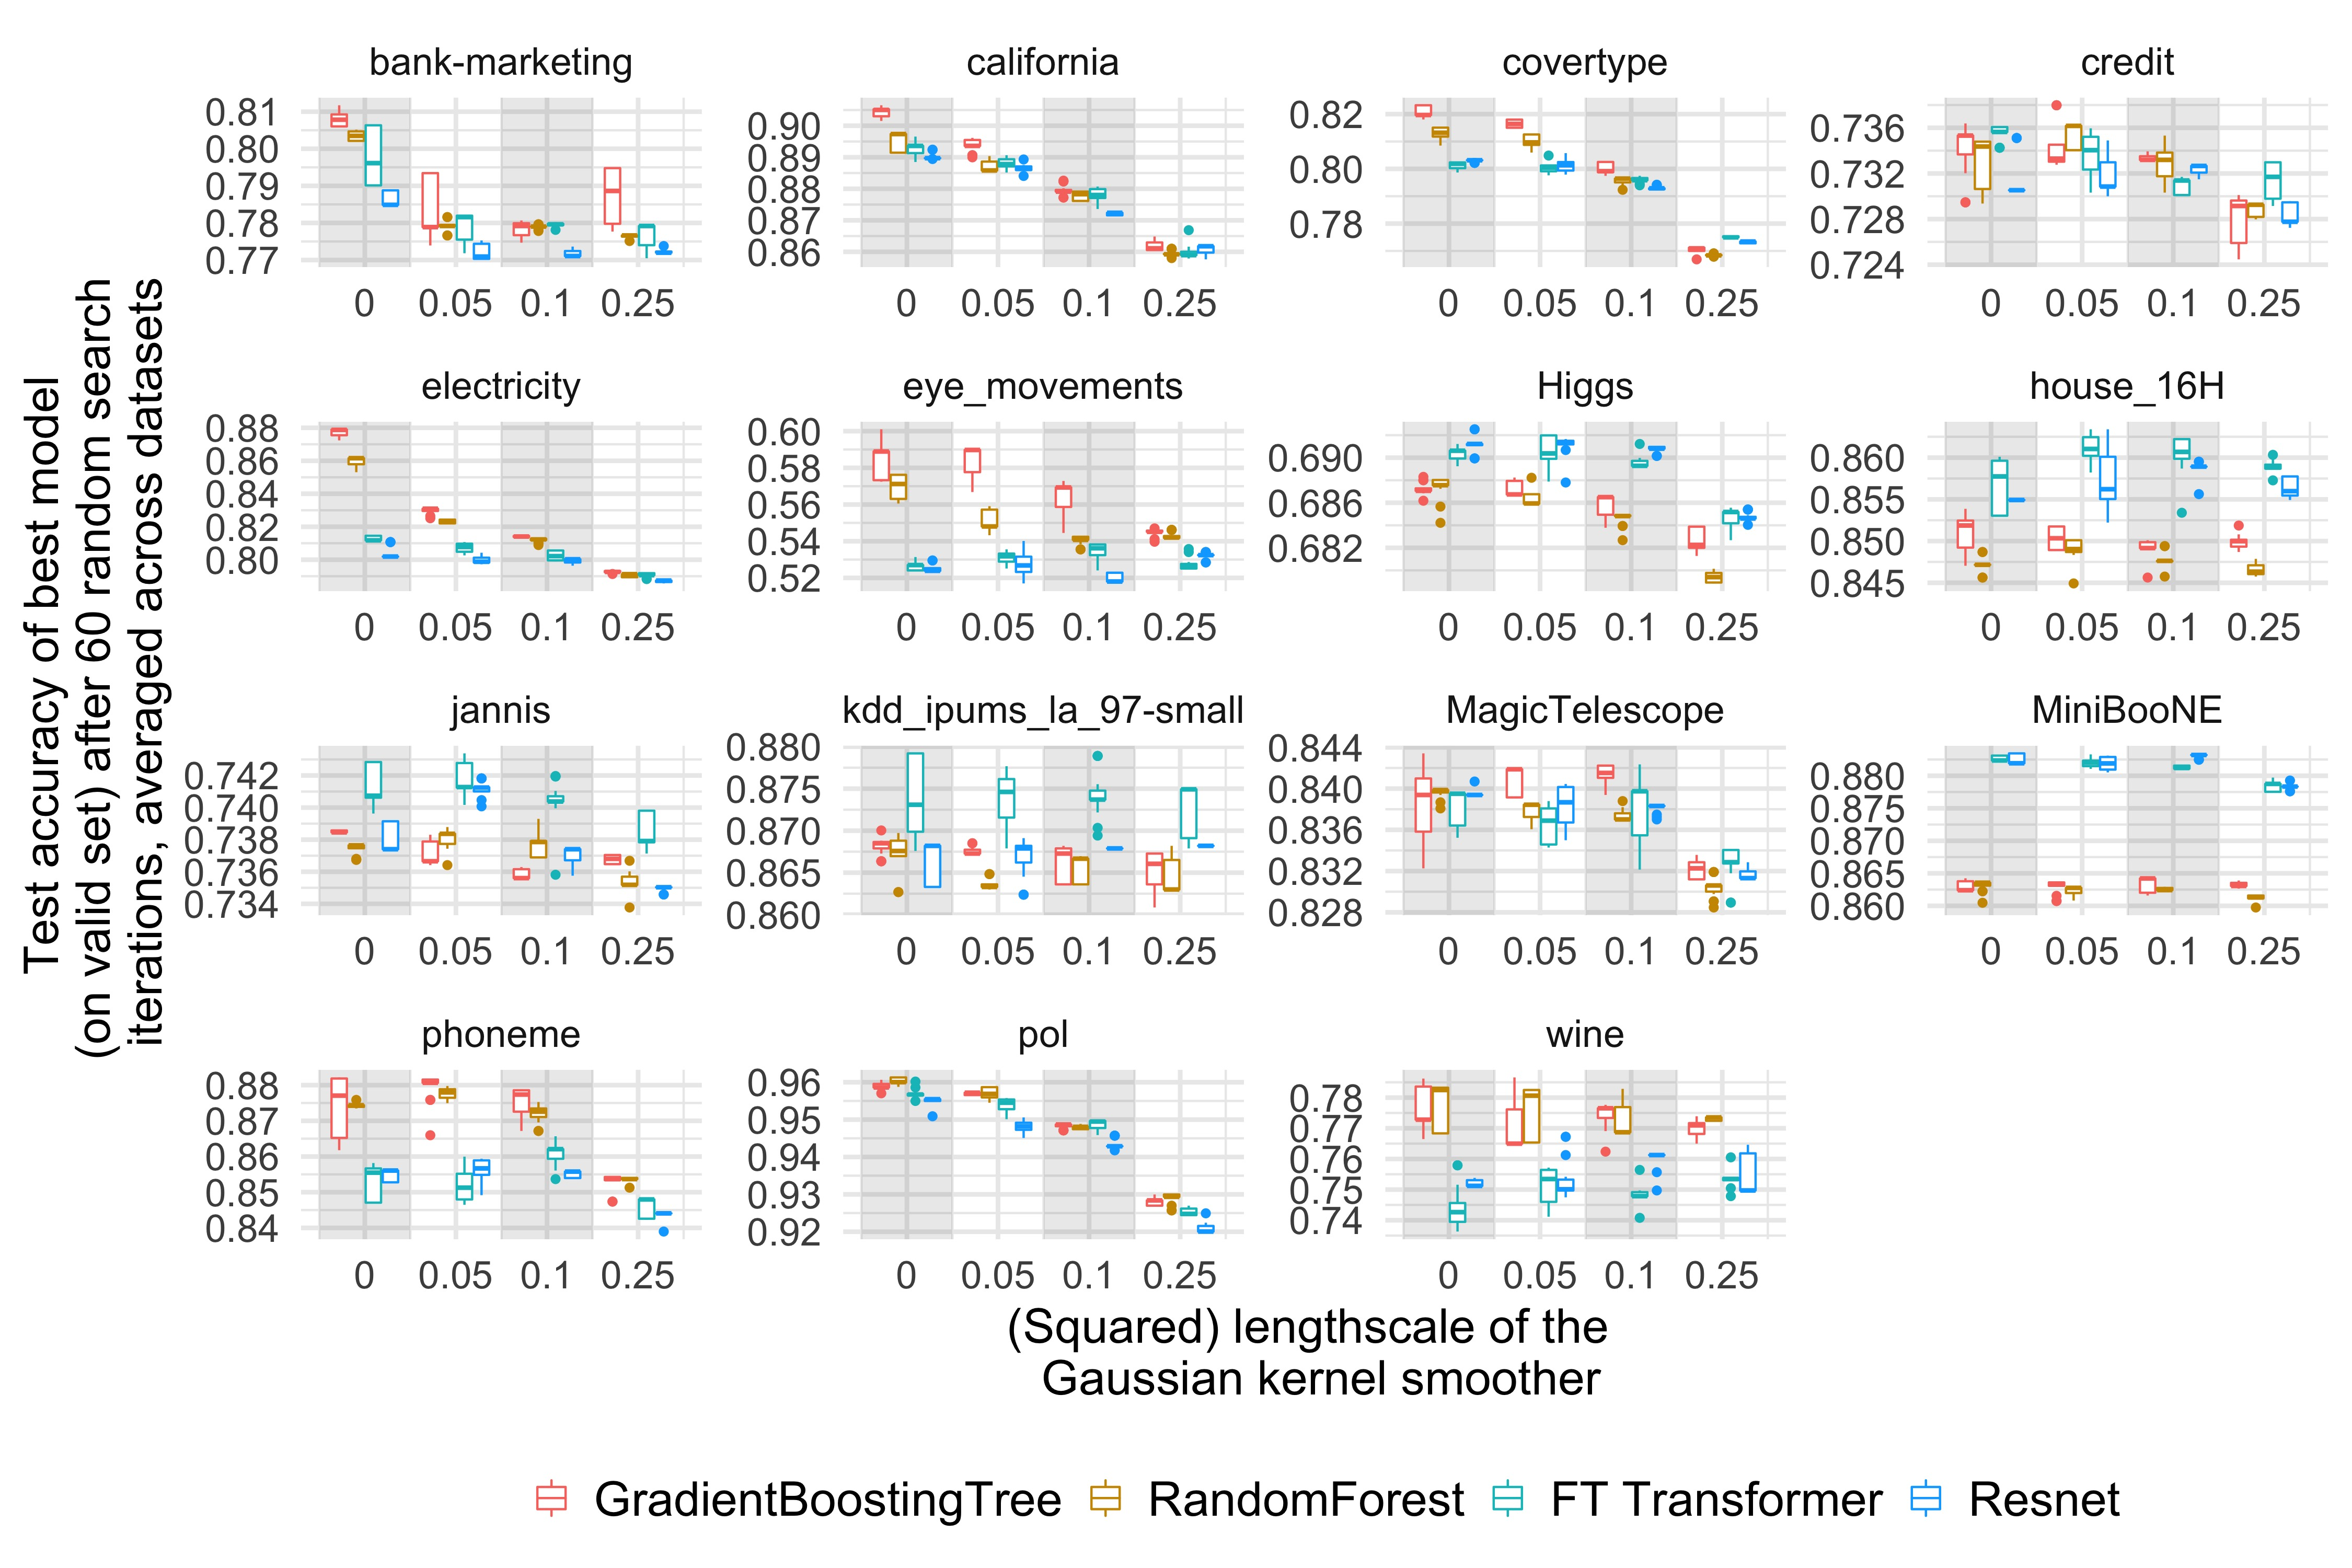}
    \caption{Same experiment than Fig. \ref{fig:high_frequencies}, shown for each dataset, without score normalization}
    \label{fig:high_frequency_dataset}
\end{figure}

Show example of decision boundaries for the best NNs vs tree-based models.

\subsection{Do our benchmarks depend on the hyperparameters sample space?}\label{supp:search_space}

For a given n, select the best order of n hp to try and then compare.

\subsection{How to use our benchmark?}\label{supp:howto}
